# Supplementary material for: Odd Viscosity and Odd Elasticity
Source: arXiv:2207.00071 source file (2022-06-30)
Supplement: Supplementary file 1 [file SupplementalInformation.pdf]

# Supplementary Information

## A. Eulerian vs Lagrangian Coordinates

This section reviews the kinematics of material deformation [1, 2]. Suppose we have a $d$-dimensional material embedded in $d$-dimensional Euclidean space $\mathbb{E}^d$. We can label each point in the material by a label $q = (q^1, q^2, \ldots, q^d) \in \mathbb{R}^d$, and we will let $\mathbf{x}(q,t) \in \mathbb{E}^d$ be the position of the material point $q$ at time $t$. For the purposes of elasticity, we will also define an arbitrary point in space defining the "undeformed" state, denoted $\mathbf{y}(q) \in \mathbb{E}^d$ (see Fig. 1). The coordinate system induces a distinguished set of basis vectors $\mathbf{x}_i = \frac{\partial \mathbf{x}}{\partial q^i}$ and $\mathbf{y}_i = \frac{\partial \mathbf{y}}{\partial q^i}$, as well as their duals $\mathbf{x}^i$ and $\mathbf{y}^i$ defined such that $\mathbf{x}^i \cdot \mathbf{x}_j = \delta^i_j$ and $\mathbf{y}^i \cdot \mathbf{y}_j = \delta^i_j$. Given an arbitrary tensor field $\mathbf{T}(q)$, we will make use of the following derivatives

$$\operatorname{Grad}\mathbf{T} = \frac{\partial \mathbf{T}}{\partial q^i} \otimes \mathbf{x}^i \qquad \operatorname{grad}\mathbf{T} = \frac{\partial \mathbf{T}}{\partial q^i} \otimes \mathbf{y}^i \tag{1}$$

$$\operatorname{Div}\mathbf{T} = \frac{\partial \mathbf{T}}{\partial q^i} \cdot \mathbf{x}^i \qquad \operatorname{div}\mathbf{T} = \frac{\partial \mathbf{T}}{\partial q^i} \cdot \mathbf{y}^i \tag{2}$$

where the sums over repeated indices are taken, $(\mathbf{a} \otimes \mathbf{b})_{\alpha\beta} = a_\alpha b_\beta$ is the direct product, and $(\mathbf{a} \cdot \mathbf{b}) = a_\alpha b_\alpha$ is the inner product, and $\alpha$, $\beta$ label the components of an orthonormal basis on $\mathbb{E}^d$. The deformation tensor is defined as the Jacobian $\mathbf{J}(q,t) = \operatorname{grad}\mathbf{x}(q,t) = \mathbf{x}_i \otimes \mathbf{y}^i$ and we will let $J = \det \mathbf{J}$. We will also define a displacement field $\mathbf{u}(q,t) = \mathbf{x}(q,t) - \mathbf{y}(q)$ and the displacement gradient $\operatorname{grad}\mathbf{u}$. Notice that $\mathbf{J}(q,t) = \mathbf{I} + \operatorname{grad}\mathbf{u}$, where $\mathbf{I}$ is the identity tensor.

For an arbitrary function $h(q,t)$, we will introduce the notation $\overline{h}(\mathbf{y}',t) = h(q,t)\big|_{\mathbf{y}'=\mathbf{y}(q)}$ and $\underline{h}(\mathbf{x}',t) = h(q,t)\big|_{\mathbf{x}'=\mathbf{x}(q,t)}$. For example, let $\rho_0(q)$ be the mass per unit volume of the material in the undeformed state. This means that the mass of a region $\mathcal{V} \subset \mathbb{R}^d$ in the coordinate system is

$$M = \int_{\mathbf{y}(\mathcal{V})} \overline{\rho_0}(\mathbf{y}')\, \mathrm{d}\mathbf{y}' = \int_{\mathbf{x}(\mathcal{V})} \underline{\rho_0}(\mathbf{x}') J^{-1} \mathrm{d}\mathbf{x}'. \tag{3}$$

We see from the Eq. (3) that the mass density of the deformed material is given by $\rho(q,t) = \rho_0(q)/J(q,t)$. Moreover, notice that

$$\operatorname{grad} h(q,t) = \nabla \overline{h}(\mathbf{y},t)\bigg|_{\mathbf{y}=\mathbf{y}(q)} \tag{4}$$

$$\operatorname{Grad} h(q,t) = \nabla \underline{h}(\mathbf{x},t)\bigg|_{\mathbf{x}=\mathbf{x}(q,t)}. \tag{5}$$

Given a Cartesian coordinate system $(r^1, \ldots, r^d)$ for $\mathbb{E}^d$, the symbol $\nabla$ acting on a function $h(\mathbf{r})$ is defined via $\nabla h(\mathbf{r}) = \frac{\partial h}{\partial r^\alpha} \hat{\mathbf{r}}_\alpha$ where $\hat{\mathbf{r}}_\alpha$ is the unit vector in the direction $r^\alpha$. Moreover,

$$\partial_t h(q,t) = \partial_t \overline{h}(\mathbf{y},t)\bigg|_{\mathbf{y}=\mathbf{y}(q,t)} \tag{6}$$

$$\partial_t g(q,t) = \partial_t \underline{h}(\mathbf{x},t) + \underline{\mathbf{v}}(\mathbf{x},t) \cdot \nabla \underline{h}(\mathbf{x},t)\bigg|_{\mathbf{x}=\mathbf{x}(q,t)} \tag{7}$$

where $\mathbf{v}(q,t) = \partial_t \mathbf{x}(q,t)$ is the velocity field. Equations expressed in terms of $\mathbf{y}$ are written in Lagrangian coordinates and equations expressed in terms of $\mathbf{x}$ are written in terms of Eulerian coordinates.

Newton's second law may be expressed in terms of the coordinates $q$ as

$$\rho_0 \partial_t \mathbf{v}(q,t) = \mathbf{f}(q,t) \tag{8}$$

where $\mathbf{f}(q,t)$ is the force per unit volume, with the volume measured in the undeformed reference state. In Lagrangian coordinates, Newton's second law reads:

$$\overline{\rho_0}(\mathbf{y}) \partial_t \overline{\mathbf{v}}(\mathbf{y},t) = \overline{\mathbf{f}}(\mathbf{y},t) \tag{9}$$

and Newton's second law in Eulerian coordinates reads:

$$\underline{\rho}[\partial_t \underline{\mathbf{v}}(\mathbf{x},t) + \underline{\mathbf{v}}(\mathbf{x},t)\cdot\nabla\underline{\mathbf{v}}(\mathbf{x},t)] = \underline{\mathbf{F}}(\mathbf{x},t). \tag{10}$$

where $\mathbf{F} = \mathbf{f}/J$ is the force per unit volume in physical space.

The flow of momentum through a solid or a fluid is described by a stress tensor. Two useful versions of the stress tensor are the Cauchy stress tensor $\boldsymbol{\sigma}(q,t)$ and the (first) Piola-Kirchhoff stress tensor $\mathbf{P}(q,t)$. Their definitions are best illustrated graphically. Consider the infinitesimal line element $\mathrm{d}q$ shown in Fig. 1, and let $\mathbf{y}(\mathrm{d}q) = \mathrm{d}\boldsymbol{\ell}$ and $\mathbf{x}(\mathrm{d}q) = \mathrm{d}\mathbf{L}$ be the image of $\mathrm{d}q$ in the underformed and deformed materials, respectively. We define unit normal vectors $\hat{\mathbf{n}} = \frac{\boldsymbol{\epsilon}\cdot\mathrm{d}\boldsymbol{\ell}}{|\mathrm{d}\boldsymbol{\ell}|}$ and $\hat{\mathbf{N}} = \frac{\boldsymbol{\epsilon}\cdot\mathrm{d}\mathbf{L}}{|\mathrm{d}\mathbf{L}|}$ to the line elements $\mathrm{d}\mathbf{L}$ and $\mathrm{d}\boldsymbol{\ell}$, respectively. Then $|\mathrm{d}\boldsymbol{\ell}|\mathbf{P}\cdot\hat{\mathbf{n}}$ represents the amount of momentum per unit time, per unit area (in the underformed material) that flows across the line element $\mathrm{d}q$. The quantity $|\mathrm{d}\mathbf{L}|\boldsymbol{\sigma}\cdot\hat{\mathbf{N}}$ represents the amount of momentum per unit time, per unit area (in real space) that flows across the line element $\mathrm{d}q$. The two stresses have the following property: $\mathbf{f}(q,t) = \operatorname{div}\mathbf{P}(q,t)$ and $\mathbf{F}(q,t) = \operatorname{Div}\boldsymbol{\sigma}(q,t)$. In Lagrangian coordinates, this reads $\overline{\mathbf{f}}(\mathbf{y},t) = \nabla\cdot\overline{\mathbf{P}}(\mathbf{y},t)$. In Eulerian coordinates, this reads $\underline{\mathbf{F}}(\mathbf{x},t) = \nabla\cdot\underline{\boldsymbol{\sigma}}(\mathbf{x},t)$. One can convert between the two tensors as follows

$$\mathbf{P} = J\boldsymbol{\sigma}\cdot\mathbf{J}^{-T} \tag{11}$$

where $\mathbf{J}^{-T}$ denotes the inverse transpose. To derive Eq. (11), it is useful to note that $\operatorname{Grad}\mathbf{T} = (\operatorname{grad}\mathbf{T})\cdot\mathbf{J}^{-1}$ for an arbitrary tensor $\mathbf{T}$, and $\operatorname{div}(J\mathbf{J}^{-T}) = 0$, which is known as the Piola identity.

Suppose $\operatorname{grad}\mathbf{u}$ is on the order of $\varepsilon \ll 1$. Then we can consider linear constitutive relations of the form

$$\boldsymbol{\sigma} = \boldsymbol{\sigma}^0 + \mathbf{C} : \operatorname{grad}\mathbf{u} + \mathcal{O}(\varepsilon^2) \tag{12}$$

$$\mathbf{P} = \mathbf{P}^0 + \mathbf{C}^{\mathrm{PK}} : \operatorname{grad}\mathbf{u} + \mathcal{O}(\varepsilon^2) \tag{13}$$

where $\boldsymbol{\sigma}^0$ and $\mathbf{P}^0$ are pre-stresses and $\mathbf{C}$ and $\mathbf{C}^{\mathrm{PK}}$ are elastic modulus tensors. Then evaluating Eq. (11) to linear order in $\varepsilon$ yields:

$$\mathbf{P} = \boldsymbol{\sigma}^0 + \boldsymbol{\sigma}\operatorname{div}\mathbf{u} - \boldsymbol{\sigma}^0\cdot(\operatorname{grad}\mathbf{u})^T + \mathbf{C} : \operatorname{grad}\mathbf{u} + \mathcal{O}(\varepsilon^2) \tag{14}$$

Defining $\boldsymbol{\sigma}^0 = \sigma^0_{ij}\,\mathbf{y}^i\otimes\mathbf{y}^j$, $\mathbf{C} = C_{ijkl}\,\mathbf{y}^i\otimes\mathbf{y}^j\otimes\mathbf{y}^k\otimes\mathbf{y}^l$, $\mathbf{C}^{\mathrm{PK}} = C^{\mathrm{PK}}_{ijkl}\,\mathbf{y}^i\otimes\mathbf{y}^j\otimes\mathbf{y}^k\otimes\mathbf{y}^l$, and $g_{ij} = \mathbf{y}_i\cdot\mathbf{y}_j$, we we obtain the conversion rule between $C_{ijkl}$ and $C^{\mathrm{PK}}_{ijkl}$ given in Section 3 of the main text:

$$C^{\mathrm{PK}}_{ijkl} = C_{ijkl} + \sigma^0_{ij}g_{kl} - \sigma^0_{il}g_{jk} \tag{15}$$

Throughout the main text, we omit the $\overline{*}$ and $\underline{*}$ notation for readability. In Section 2, all equations are written in Eulerian coordinates and in Section 3, all equations are in Lagrangian coordinates.

## B. Rank two and four isotropic tensors

Here we review a few basic facts about rank-2 and rank-4 isotropic tensors in two dimensions. Let $T_{ij}$ be a rank two tensor, say the stress, strain, or velocity gradient tensor. When we perform a passive rotation of the coordinate system, $T_{ij}$ transforms as $\tilde{T}_{ij} = R_{ik}(\theta)R_{jl}(\theta)T_{kl}$, where $R_{ij} = \cos\theta\delta_{ij} + \sin\theta\epsilon_{ij}$ is a rotation matrix. It is useful to introduce the following basis for two by two matrices:

$$\tau^0_{ij} = \delta_{ij} \qquad \tau^1_{ij} = -\epsilon_{ij} \qquad \tau^2_{ij} = \begin{pmatrix}1 & 0\\ 0 & -1\end{pmatrix} \qquad \tau^3_{ij} = \begin{pmatrix}0 & 1\\ 1 & 0\end{pmatrix} \tag{16}$$

Then we may define $T_\alpha = \tau^\alpha_{ij}T_{ij}$. Notice that this implies $T_{ij} = \frac{1}{2}T_\alpha\tau^\alpha_{ij}$ since $\tau^\alpha_{ij}\tau^\beta_{ij} = 2\delta_{\alpha\beta}$. Under rotations, one finds $\tilde{T}_\alpha = R_{\alpha\beta}T_\beta$, where

$$R_{\alpha\beta} = \frac{1}{2}\tau^\alpha_{ij}\tau^\beta_{k\ell}R_{ik}R_{j\ell} = \begin{pmatrix}1 & 0 & 0 & 0\\ 0 & 1 & 0 & 0\\ 0 & 0 & \cos 2\theta & \sin 2\theta\\ 0 & 0 & -\sin 2\theta & \cos 2\theta\end{pmatrix} \tag{17}$$

A tensor $T_{ij}$ is said to be isotropic (i.e. invariant under $SO(2)$) if $\tilde{T}_{ik} = T_{ij}$ for all $\theta$. From Eq. (17), we see that isotropy implies $T_2 = T_3 = 0$. In other words, only the trace and antisymmetric part of 2D matrices are invariant under rotations.

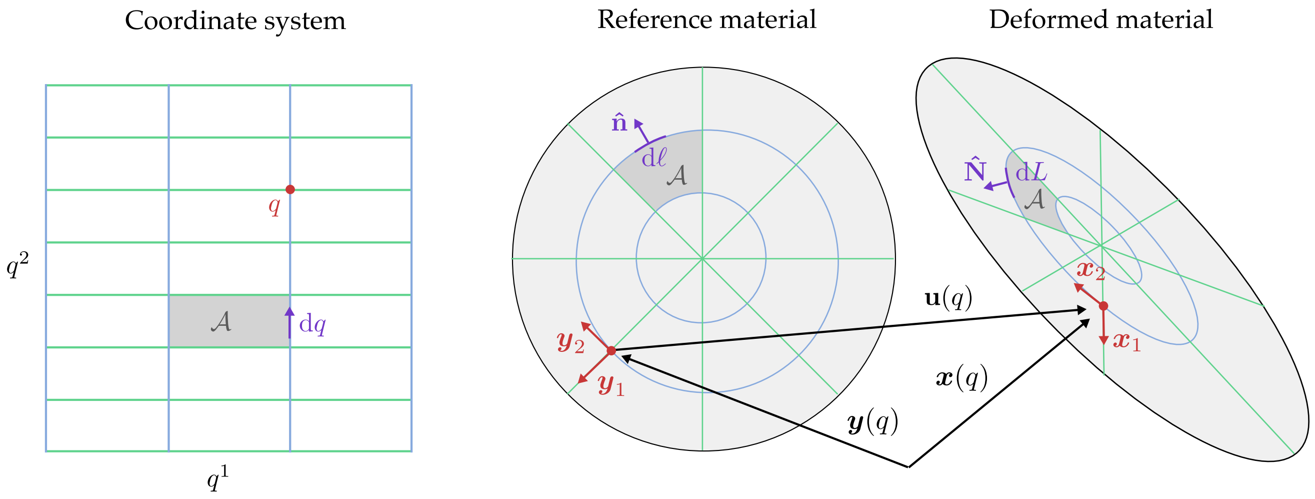


FIG. 1. An illustration of the coordinate systems defined in Section A. Adapted from [3].

A similar result holds for rank four tensors $M_{ijk\ell}$. Thinking of $M_{ijk\ell}$ as a linear map between rank two tensors, it is useful to define

$$M_{\alpha\beta} = \frac{1}{4}\tau^{\alpha}_{ij}\tau^{\beta}_{k\ell}M_{ijk\ell} \tag{18}$$

In this case, under rotations, we have $\tilde{M}_{ijk\ell} = R_{im}R_{jn}R_{kp}R_{\ell q}M_{mnpq}$, or equivalently $\tilde{M}_{\alpha\beta} = R_{\alpha\gamma}R_{\beta\sigma}M_{\gamma\sigma}$. By explicitly writing out the matrix multiplication between four-by-four matrices, one can verify that the most general four-by-four matrix with $\tilde{M}_{\alpha\beta} = M_{\alpha\beta}$ for all $\theta$ takes the form:

$$M_{\alpha\beta} = \begin{pmatrix} M_{00} & M_{01} & 0 & 0 \\ M_{10} & M_{11} & 0 & 0 \\ 0 & 0 & M_{22} & M_{23} \\ 0 & 0 & -M_{23} & M_{22} \end{pmatrix} \tag{19}$$

Then utilizing the relationship $M_{ijk\ell} = \tau^{\alpha}_{ij}\tau^{\beta}_{k\ell}M_{\alpha\beta}$

$$\begin{aligned} M_{ijk\ell} =& M_{00}\delta_{ij}\delta_{k\ell} + M_{22}\left(\delta_{i\ell}\delta_{jk} + \delta_{ik}\delta_{j\ell} - \delta_{ij}\delta_{k\ell}\right) - M_{10}\epsilon_{ij}\delta_{k\ell} \\ &+ M_{23}(\epsilon_{ik}\delta_{j\ell} + \epsilon_{j\ell}\delta_{ik}) - M_{01}\delta_{ij}\epsilon_{k\ell} + M_{11}\epsilon_{ij}\epsilon_{k\ell} \end{aligned} \tag{20}$$

The above discussion yields the form of the 2D elastic modulus and viscosity tensors used in the main text. In particular, we define $e_\alpha = \tau^{\alpha}_{ij}\partial_i u_j$, $\dot{e}_\alpha = \tau^{\alpha}_{ij}\partial_i v_j$, and $\sigma_\alpha = \frac{1}{2}\tau^{\alpha}_{ij}\sigma_{ij}$ (note the factor of two). The elasticity and viscosity matrix are given by $C_{\alpha\beta} = \frac{1}{4}\tau^{\alpha}_{ij}\tau^{\beta}_{k\ell}C_{ijk\ell}$ and $\eta_{\alpha\beta} = \frac{1}{4}\tau^{\alpha}_{ij}\tau^{\beta}_{k\ell}\eta_{ijk\ell}$.

---

[1] Zubov, L. *Nonlinear Theory of Dislocations and Disclinations in Elastic Bodies*. Lecture Notes in Physics Monographs (Springer Berlin Heidelberg, 2008).

[2] Marsden, J. E. *Mathematical foundations of elasticity* (Dover, New York, 1994). Originally published: Englewood Cliffs, N.J. : Prentice-Hall, c1983.

[3] Braverman, L., Scheibner, C., VanSaders, B. & Vitelli, V. Topological defects in solids with odd elasticity. *Physical Review Letters* **127**, 268001 (2021).
